# Supplementary material for: Direct visualization and control of antiferromagnetic domains and spin reorientation in a parent cuprate
Source: arXiv:2210.04327 source file (2022-10-09)
Supplement: Supplementary file 1 [file supplement.pdf]

# Supplementary Information: Direct visualization and control of antiferromagnetic domains and spin reorientation in a parent cuprate

K. L. Seyler, A. Ron, D. Van Beveren, C. R. Rotundu, Y. S. Lee, and D. Hsieh

**Contents**

1. Experimental methods 2
2. Analysis of the SHG processes 3
3. RA-SHG above and below $T_{\mathrm{N,I}}$ 6
4. Thermal cycling studies and magnetic domains in free-standing sample 7
5. Magnetic field dependence of domains at room temperature 8
6. Comparison to conclusions drawn from prior magnetization experiments 9
7. Full temperature dependence of magnetic domains 10
8. Observation of domain reorientation transition in an additional sample 11
9. Field-direction dependence of single-domain magnetization near $T_{\mathrm{R}}$ 12
References 13

## 1. Experimental methods

$Sr_2Cu_3O_4Cl_2$ crystals were grown by an optimized method of slow cooling from the melt [1]. Quantities of SrO, $SrCl_2$, and CuO powders were mixed in a 1:1:3 stoichiometric ratio and placed in a large high form alumina crucible. The mix was gradually heated in air 1030 °C, dwelled for 5 h, then cooled to 900 °C at a rate of 2 °C $h^{-1}$. Placing the crucible in a slight temperature gradient (off-center of the hot chamber of the box furnace) resulted in a cm-sized plate-like single crystal. Samples are stable in air. High quality of the samples was attested by X-ray diffraction, Laue X-ray, and low-temperature magnetization measurements. The samples were affixed to an oxygen-free high thermal conductivity copper mount using a small amount of epoxy and then cleaved before measurement to leave clean surfaces parallel to the $Cu_3O_4$ (001) planes.

RA-SHG measurements were carried out using a rotating scattering plane based technique [2] with laser pulses at a fundamental wavelength of 800 nm delivered by a Ti:sapphire amplifier (∼80 fs pulse duration, 100 kHz repetition rate). The experimental geometry is depicted in Fig. 1b. The beam diameter was ∼40 µm with a fluence ∼3 mJ/$cm^2$. For oblique incidence data, the angle of incidence was $\theta = 10°$.

Wide-field imaging was performed with linear polarized excitation at $\theta \approx 0°$ with a fluence of ∼1 mJ/$cm^2$ unless otherwise specified. The excitation spot size was ∼200 µm for Fig. 1g and ∼500 µm for all other figures. The direction of the linear polarization for each dataset, which determines whether a particular domain is bright or dark, is indicated in the respective figure captions. The intensity fall-off near the edges of the image is an artefact due to the intensity profile of the excitation beam; $\mathbf{M}$ does not vary appreciably within a single domain at a given temperature. Additional bright or dark lines in the SHG image arise from scattering off the terrace edges. Significantly higher average power was required for SHG imaging (typically ∼100 mW) compared to RA-SHG (∼3 mW) due to the larger illumination area, which causes additional sample heating. The temperature values reported in Fig. 3a and Fig. 4 are corrected for this laser heating by comparing low-power (0.5 mW) RA-SHG data on domain B to the SHG images.

The magnetic-field-dependent measurements (AM-SHG and field-dependent SHG imaging) were performed using home-built permanent magnet setups (neodymium for room-temperature or SmCo for low-temperature studies). The magnetic field direction and magnitude were controlled by adjusting the permanent magnet positions with translation and rotation stages, and the setup was calibrated with a gauss meter.

To determine the domain wall positions for Fig. 4, a linecut was performed along the $y$ direction in each SHG image after averaging 16 $x$ pixels. The position was then determined from the derivative of the linecut after applying a Savitzky-Golay filter. The spatial resolution was limited by the pixel size (∼4.2 µm), which was used as the uncertainty of the domain wall position.

## 2. Analysis of the SHG processes

In this section, we provide a mathematical description of the SHG response. Above $T_{\mathrm{N,I}}$, $\mathrm{Sr_2Cu_3O_4Cl_2}$ possesses a centrosymmetric tetragonal structure (point group $4/mmm$), so the bulk electric dipole (ED) response vanishes. Surface ED (point group $4mm$) as well as bulk magnetic dipole (MD) $i$-type processes are allowed, but these terms are $\varphi$-independent in the $\mathrm{P_{out}}$ channels and zero in the $\mathrm{S_{out}}$ channels [3]. This is incompatible with our experiments (Fig. S1), so we exclude such contributions. SHG can also arise from an electric quadrupole (EQ) process ($\chi^{\mathrm{EQ}(i)}$) from $4/mmm$, similar to what occurs in $\mathrm{Sr_2CuO_2Cl_2}$ [3]. This process has the form $P_i^{2\omega} = \chi_{ijkl}^{\mathrm{EQ}(i)} E_j^{\omega}(\partial_k E_l^{\omega} + \partial_l E_k^{\omega})$, where $\mathbf{P}^{2\omega}$ is the second-harmonic polarization at frequency $2\omega$, $\mathbf{E}^{\omega}$ is the electric field at the fundamental frequency $\omega$, and the indices $i, j, k, l$ run over the coordinates $x, y, z$. The bulk EQ SHG intensity has $|a + b\cos 4\varphi|^2$ dependence (where $a$ and $b$ are constants) for $\mathrm{P_{out}}$ channels and $|\sin 4\varphi|^2$ dependence for $\mathrm{S_{out}}$ channels, consistent with our observations. In fact, the $\mathrm{Sr_2Cu_3O_4Cl_2}$ SHG is similar to $\mathrm{Sr_2CuO_2Cl_2}$ in not only symmetry but also intensity, which suggests that they share a common SHG origin. For $\mathrm{Sr_2CuO_2Cl_2}$, it was proposed that the EQ SHG is enhanced by an EQ $d$-$d$ transition at the fundamental energy (1.5 eV) [3, 4], so the same resonant SHG process likely also occurs in $\mathrm{Sr_2Cu_3O_4Cl_2}$. The full $i$-type (time invariant) rank-4 polar susceptibility tensor $\chi^{\mathrm{EQ}(i)}$ and the EQ SHG expressions for $4/mmm$ are detailed thoroughly in Ref. [3].

Below $T_{\mathrm{N,I}}$, where the $\mathrm{Cu_I}$ spins antiferromagnetically order and the $\mathrm{Cu_{II}}$ spins become polarized due to the pseudodipolar interaction, $\mathrm{Sr_2Cu_3O_4Cl_2}$ possesses the magnetic point group $mm'm'$. The two lowest order processes that become allowed below $T_{\mathrm{N,I}}$ are $c$-type (time-noninvariant) bulk MD SHG ($\chi^{\mathrm{MD}(c)}$) and $c$-type surface ED SHG ($\chi_{\mathrm{s}}^{\mathrm{ED}(c)}$). We first describe the MD case, and then we will discuss the surface ED process and why it is likely weak relative to the MD process. The MD process may be written as $P_i^{2\omega} = \chi_{ijk}^{\mathrm{MD}(c)} E_j^{\omega} H_k^{\omega}$ where $\mathbf{H}^{\omega}$ is the fundamental-frequency magnetic field and $\chi^{\mathrm{MD}(c)}$ is the $c$-type rank-3 axial susceptibility tensor that that respects $mm'm'$. The data show the onset of a magnetic SHG process that is linearly related to the ferromagnetic moment $\mathbf{M}$. We therefore expand the susceptibility as $\chi^{\mathrm{MD}(c)}(\mathbf{M}) = \chi_{0,ijk}^{\mathrm{MD}} + \chi_{ijkl} M_l$. The first term (H3 in Birss [5]) represents a crystallographic contribution (independent of magnetic order) that gives $\varphi$-independent SHG response [3] contrary to our observations and can therefore be neglected. $\chi_{ijkl}$ is an $i$-type rank-4 polar tensor that respects the crystallographic point group of the paramagnetic phase. Under tetragonal symmetry, $\chi_{ijkl}$ possesses the following form (H4 in Birss [5])

$$\chi_{ijkl} = \begin{pmatrix} \begin{pmatrix} \chi_{xxxx} & 0 & 0 \\ 0 & \chi_{xxyy} & 0 \\ 0 & 0 & \chi_{xxzz} \end{pmatrix} & \begin{pmatrix} 0 & \chi_{xyxy} & 0 \\ \chi_{xyyx} & 0 & 0 \\ 0 & 0 & 0 \end{pmatrix} & \begin{pmatrix} 0 & 0 & \chi_{xzxz} \\ 0 & 0 & 0 \\ \chi_{xzzx} & 0 & 0 \end{pmatrix} \\ \begin{pmatrix} 0 & \chi_{xyyx} & 0 \\ \chi_{xyxy} & 0 & 0 \\ 0 & 0 & 0 \end{pmatrix} & \begin{pmatrix} \chi_{xxyy} & 0 & 0 \\ 0 & \chi_{xxxx} & 0 \\ 0 & 0 & \chi_{xxzz} \end{pmatrix} & \begin{pmatrix} 0 & 0 & 0 \\ 0 & 0 & \chi_{xzxz} \\ 0 & \chi_{xzzx} & 0 \end{pmatrix} \\ \begin{pmatrix} 0 & 0 & \chi_{zxxz} \\ 0 & 0 & 0 \\ \chi_{zxzx} & 0 & 0 \end{pmatrix} & \begin{pmatrix} 0 & 0 & 0 \\ 0 & 0 & \chi_{zxxz} \\ 0 & \chi_{zxzx} & 0 \end{pmatrix} & \begin{pmatrix} \chi_{zzxx} & 0 & 0 \\ 0 & \chi_{zzxx} & 0 \\ 0 & 0 & \chi_{zzzz} \end{pmatrix} \end{pmatrix}. \qquad (1)$$

In general, these tensor elements are complex. Using the in-plane ferromagnetic moment, $\mathbf{M} = (M_x, M_y, 0)$, we may

write the following susceptibility tensor for the MD SHG process

$$\chi_{ijk}^{\mathrm{MD}(c)}(\mathbf{M}) = \chi_{ijkl}M_l = \begin{pmatrix} \begin{pmatrix} M_x\chi_{xxxx} \\ M_y\chi_{xxyy} \\ 0 \end{pmatrix} & \begin{pmatrix} M_y\chi_{xyxy} \\ M_x\chi_{xyyx} \\ 0 \end{pmatrix} & \begin{pmatrix} 0 \\ 0 \\ M_x\chi_{xzzx} \end{pmatrix} \\ \begin{pmatrix} M_y\chi_{xyyx} \\ M_x\chi_{xyxy} \\ 0 \end{pmatrix} & \begin{pmatrix} M_x\chi_{xxyy} \\ M_y\chi_{xxxx} \\ 0 \end{pmatrix} & \begin{pmatrix} 0 \\ 0 \\ M_y\chi_{xzzx} \end{pmatrix} \\ \begin{pmatrix} 0 \\ 0 \\ M_x\chi_{zxzx} \end{pmatrix} & \begin{pmatrix} 0 \\ 0 \\ M_x\chi_{zxzx} \end{pmatrix} & \begin{pmatrix} M_x\chi_{zzxx} \\ M_y\chi_{zzxx} \\ 0 \end{pmatrix} \end{pmatrix}. \tag{2}$$

The total SHG intensity below $T_{\mathrm{N,I}}$ is given by

$$I(2\omega,\phi) = |A\hat{e}_i^{\mathrm{out}}\chi_{ijkl}^{\mathrm{EQ}(i)}\hat{e}_j^{\mathrm{in}}q_k\hat{e}_l^{\mathrm{in}} + A\hat{e}_i^{\mathrm{out}}\chi_{ijk}^{\mathrm{MD}(c)}(\mathbf{M})\hat{e}_j^{\mathrm{in}}\epsilon_{klm}q_l\hat{e}_m^{\mathrm{in}}|^2 I(\omega)^2, \tag{3}$$

where $\vec{q}$ is the wavevector of incident light, $\hat{e}$ is the polarization of incoming fundamental or outgoing second-harmonic light, $I(\omega)$ is the intensity of the fundamental beam, $A$ is a constant that depends on the polarization geometry, and $\epsilon_{klm}$ is the Levi-Civita symbol. The MD contributions to the second-harmonic electric fields for the four polarization geometries are then given by

$$\begin{aligned} E_{\mathrm{PP}}^{2\omega} \propto\ & \sin^2\theta(-M_y\cos\varphi - M_x\sin\varphi)\chi_{zxzx} \\ & + \cos^2\theta\Big(-M_y\chi_{xyxy}\cos^3\varphi + M_x(-\chi_{xxxx}+\chi_{xyyx}+\chi_{xxyy})\cos^2\varphi\sin\varphi \\ & + M_y(-\chi_{xxxx}+\chi_{xyyx}+\chi_{xxyy})\cos\varphi\sin^2\varphi - M_x\chi_{xyxy}\sin^3\varphi\Big) \end{aligned} \tag{4}$$

$$\begin{aligned} E_{\mathrm{SP}}^{2\omega} \propto\ & \sin^2\theta(M_y\cos\varphi + M_x\sin\varphi)\chi_{zzxx} \\ & + \cos^2\theta\Big(M_y\chi_{xxyy}\cos^3\varphi + M_x(\chi_{xxxx}-\chi_{xyyx}-\chi_{xyxy})\cos^2\varphi\sin\varphi \\ & + M_y(\chi_{xxxx}-\chi_{xyyx}-\chi_{xyxy})\cos\varphi\sin^2\varphi + M_x\chi_{xxyy}\sin^3\varphi\Big) \end{aligned} \tag{5}$$

$$\begin{aligned} E_{\mathrm{PS}}^{2\omega} \propto\ & \cos\theta\Big(-M_x\chi_{xxyy}\cos^3\varphi + M_y(\chi_{xxxx}-\chi_{xyyx}-\chi_{xyxy})\cos^2\varphi\sin\varphi \\ & + M_x(-\chi_{xxxx}+\chi_{xyyx}+\chi_{xyxy})\cos\varphi\sin^2\varphi + M_y\chi_{xxyy}\sin^3\varphi\Big) \end{aligned} \tag{6}$$

$$\begin{aligned} E_{\mathrm{SS}}^{2\omega} \propto\ & \cos\theta\Big(M_x\chi_{xyxy}\cos^3\varphi + M_y(-\chi_{xxxx}+\chi_{xyyx}+\chi_{xxyy})\cos^2\varphi\sin\varphi \\ & + M_x(\chi_{xxxx}-\chi_{xyyx}-\chi_{xxyy})\cos\varphi\sin^2\varphi - M_y\chi_{xyxy}\sin^3\varphi\Big) \end{aligned} \tag{7}$$

In the case of normal incidence ($\theta = 0°$), the EQ contribution goes to zero, leaving MD SHG with $C_2$ symmetry in the RA intensity pattern, consistent with Fig. 1c. At oblique incidence, the nonzero EQ SHG will interfere with the MD SHG, leading to RA patterns with $C_1$ symmetry, consistent with our observations (Fig. S1). We note that to achieve good fits to the magnetic-field-dependent RA patterns in Fig. 2a, we must assume that $\chi_{ijkl}$ respects orthorhombic symmetry. In this case, $\chi_{ijkl}$ possesses the same basic form as with the tetragonal case (Eq. 1) but more elements are independent of one another (D4 in Birss [5]). Therefore, the resulting SHG expressions are very similar but the additional independent elements allow for a different magnetic response along the $x$ and $y$ axes.

Below $T_{\mathrm{N,I}}$, a $c$-type electric dipole (ED) process, $P_i^{2\omega} = \chi_{\mathrm{s},ijk}^{\mathrm{ED}(c)} E_j^{\omega} E_k^{\omega}$, from the surface magnetic point group $m'm2'$ also becomes allowed. In this case, we proceed similar to the MD case, but $\chi_{ijkl}$ becomes an axial tensor for the surface crystallographic structure (I4 in Birss [5]). The surface ED contributions to the second-harmonic electric fields for the four polarization geometries are given by

$$\begin{aligned} E_{\mathrm{s,PP}}^{2\omega} \propto\ & \cos\theta \sin^2\theta (M_y \cos\varphi + M_x \sin\varphi)(\chi_{xzzy} + 2\chi_{zxzy}) \\ & + \cos^3\theta \Big( M_y \chi_{xxxy} \cos^3\varphi + M_x(-2\chi_{xxyx} - \chi_{yxxx}) \cos^2\varphi \sin\varphi \\ & + M_y(-2\chi_{xxyx} - \chi_{yxxx}) \cos\varphi \sin^2\varphi + M_x \chi_{xxxy} \sin^3\varphi \Big) \end{aligned} \tag{8}$$

$$\begin{aligned} E_{\mathrm{s,SP}}^{2\omega} \propto\ & \cos\theta \Big( -M_y \chi_{yxxx} \cos^3\varphi + M_x(\chi_{xxxy} + 2\chi_{xxyx}) \cos^2\varphi \sin\varphi \\ & + M_y(\chi_{xxxy} + 2\chi_{xxyx}) \cos\varphi \sin^2\varphi - M_x \chi_{yxxx} \sin^3\varphi \Big) \end{aligned} \tag{9}$$

$$\begin{aligned} E_{\mathrm{s,PS}}^{2\omega} \propto\ & \sin^2\theta (-M_x \cos\varphi + M_y \sin\varphi) \chi_{xzzy} \\ & + \cos^2\theta \Big( M_x \chi_{yxxx} \cos^3\varphi + M_y(\chi_{xxxy} + 2\chi_{xxyx}) \cos^2\varphi \sin\varphi \\ & + M_x(-\chi_{xxxy} - 2\chi_{xxyx}) \cos\varphi \sin^2\varphi - M_y \chi_{yxxx} \sin^3\varphi \Big) \end{aligned} \tag{10}$$

$$\begin{aligned} E_{\mathrm{s,SS}}^{2\omega} \propto\ & - M_x \chi_{xxxy} \cos^3\varphi - M_y(\chi_{yxxx} + 2\chi_{xxyx}) \cos^2\varphi \sin\varphi \\ & + M_x(\chi_{yxxx} + 2\chi_{xxyx}) \cos\varphi \sin^2\varphi + M_y \chi_{xxxy} \sin^3\varphi \end{aligned} \tag{11}$$

By comparing Eq. (4)–(7) and Eq. (8)–(11), we see that the $\varphi$-dependence is similar. It is therefore not surprising that bulk MD and surface ED achieve comparable fits to the data. However, prior work has shown that the susceptibility for surface-magnetization-induced ED SHG is an order of magnitude weaker than that of crystallographic surface ED in $3d$ transition metal systems [6, 7]. In addition, for $Sr_2IrO_4$, which has much stronger spin-orbit coupling and magnetic moment ($\sim 0.1\,\mu_B$/Ir), the magnetic surface ED term is still much weaker than the bulk MD term [8]. While we cannot rule out the presence of a magnetic surface ED process, this strongly suggests that the bulk magnetic MD term should dominate in $Sr_2Cu_3O_4Cl_2$.

### 3. RA-SHG above and below $T_{N,I}$

Figure S1 shows RA-SHG patterns for $P_{in}$-$P_{out}$, $S_{in}$-$P_{out}$, $P_{in}$-$S_{out}$, and $S_{in}$-$S_{out}$ channels on domain A and B above and below $T_{N,I}$. Above $T_{N,I}$, the patterns are consistent with an EQ process, $\chi^{EQ(i)}$, from the reported bulk $4/mmm$ crystal structure. Below $T_{N,I}$, all patterns are reduced to $C_1$ symmetry and fit well to a coherent superposition of a $\chi^{EQ(i)}$ process from the bulk $4/mmm$ crystal structure and a magnetization-induced $\chi^{MD(c)}$ process from the reported magnetic structure $mm'm'$. Fitting expressions are provided in Section S2.

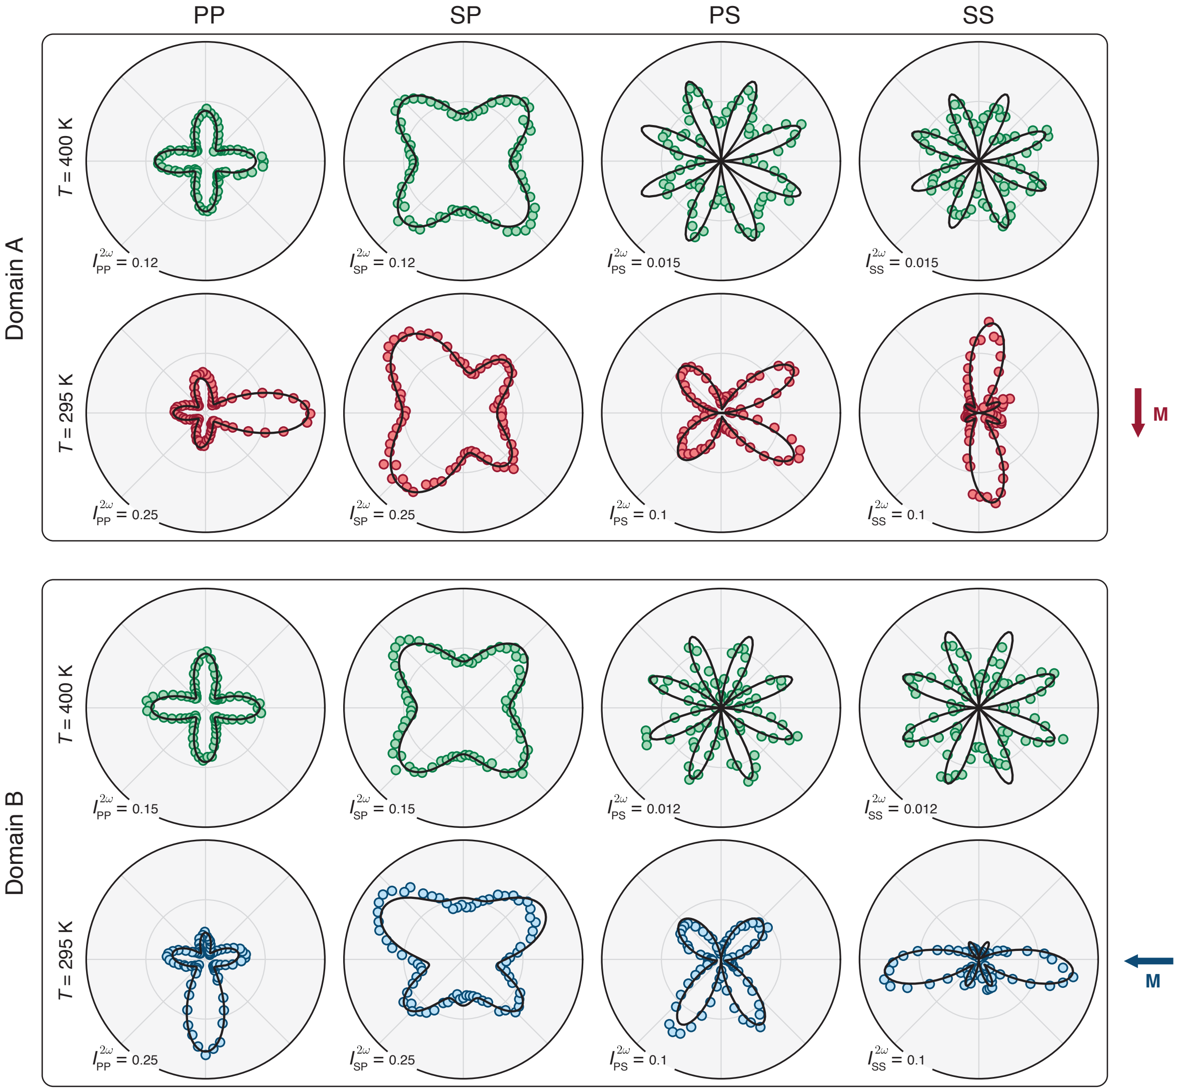


FIG. S1. RA-SHG patterns for all four polarization geometries taken above $T_{N,I}$ at 400 K and below $T_{N,I}$ at 295 K. The top (bottom) panel shows data for domain A (B). Solid curves are fits to the data using a $\chi^{EQ(i)}$ ($4/mmm$) process for above $T_{N,I}$ and coherent superposition of $\chi^{EQ(i)}$ ($4/mmm$) and $\chi^{MD(c)}$ ($mm'm'$) processes for below $T_{N,I}$. The direction of the ferromagnetic moment **M** is indicated on the right.

### 4. Thermal cycling studies and magnetic domains in free-standing sample

Figure S2 explores the origin of the magnetic domains with relative order parameter orientations of 90°. By tracking **M** at 295 K after thermal cycling through $T_{N,I}$, we determine that the Earth's magnetic field can train the moment direction in each domain (Fig. S2a). This may explain why we do not observe 180° domain walls, since they are likely very sensitive to small magnetic fields. We also observe that domains always prefer to orient along a fixed axis; changing the direction of Earth's field can flip each domain by 180° but never by 90°. The data imply the existence of a uniaxial magnetic easy axis for each domain.

Thermal cycling measurements in Fig. S2b reveal pinned domain states and domain walls after thermal cycling through $T_{N,I}$, though the particular configuration depends on the temperature as well as whether the sample has been cooled (from 400 K) or heated (from 80 K). One possibility is that the pinning effects arise from extrinsic factors, such as the stress from the sample mounting procedure. However, we also observe similar 90° domains in nearly free-standing samples (Fig. S2c), so it is likely that the pinning originates from characteristics of the samples themselves.

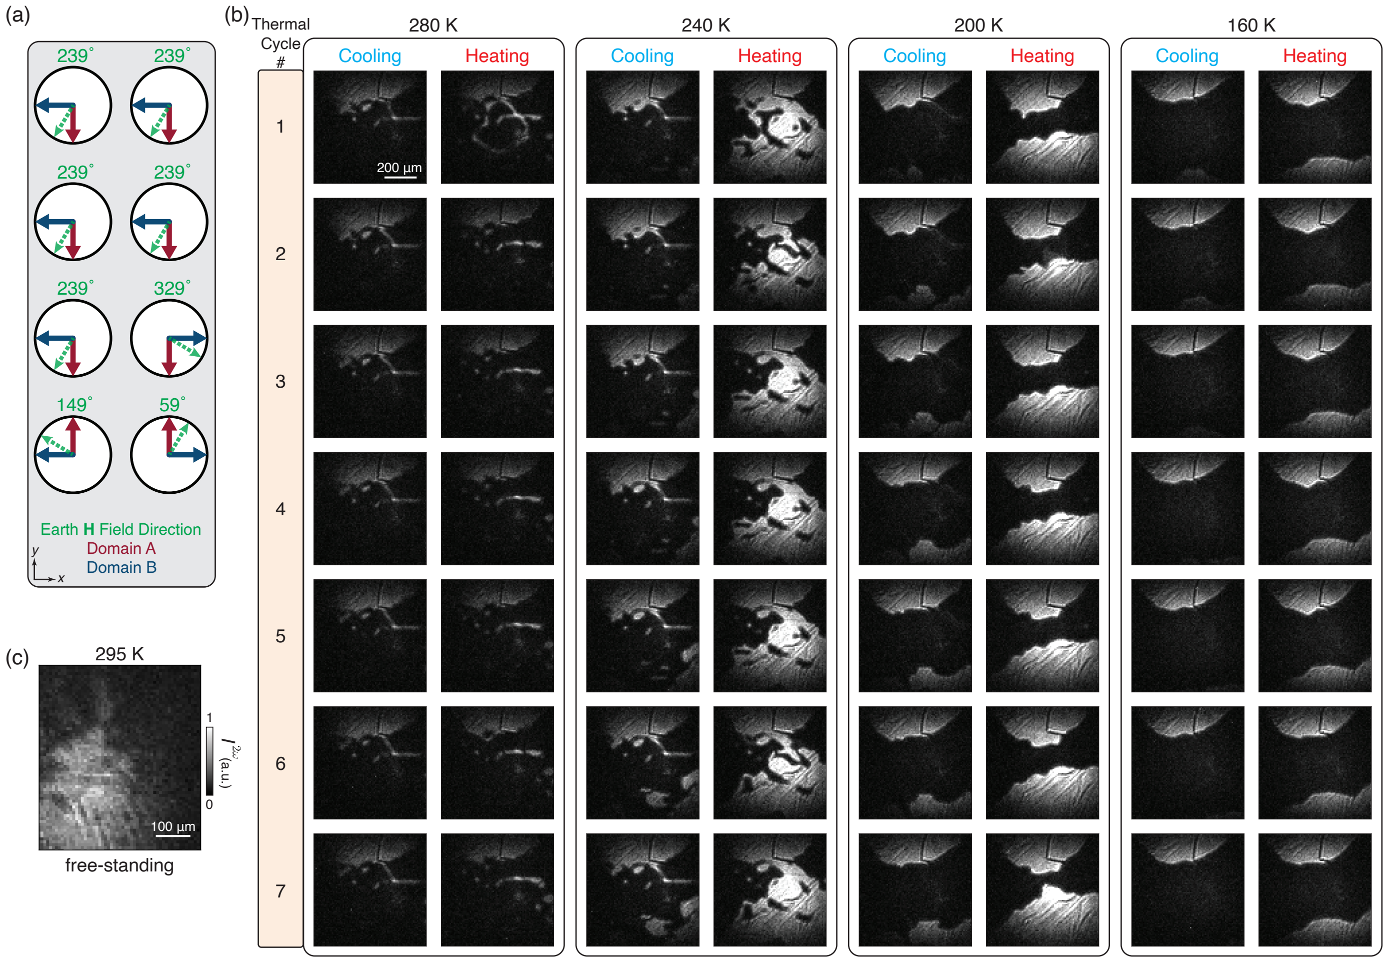


FIG. S2. **a**, Effect of thermal cycling above $T_{N,I}$ on the direction of **M** for different Earth magnetic field directions. Each circle depicts **M** of domain A (red arrow) and B (blue arrow) at 295 K after thermal cycling to 400 K using a particular direction of the ∼0.5 Oe Earth's magnetic field (dashed green arrow and labeled angle). **b**, Domain pinning after thermal cycling. Each of the four panels show SHG images at the specified temperature after cooling (left column) from 400 K or after heating from 80 K (right column) for seven different thermal cycles (rows). Images acquired with vertical excitation polarization. **c**, SHG image from a different "free-standing" $Sr_2Cu_3O_4Cl_2$ sample showing large magnetic domains at 295 K with relative magnetization directions of 90°. The sample was loosely attached to double-sided tape at 295 K to minimize stress on it.

### 5. Magnetic field dependence of domains at room temperature

Figure S3 shows how the domain structure evolves under increasing in-plane magnetic fields at 295 K. The evolution from a 90° to 0° domain appears to take place through nucleation of small domains that grow and merge. We note that the 90° domain wall position does not show appreciable motion at low fields, which indicates a larger uniaxial anisotropy and a smaller domain wall susceptibility at room temperature compared to near $T_{\mathrm{R}}$.

To obtain a rough estimate of the uniaxial anisotropy energy, one can calculate the energy needed to magnetize a domain in a direction perpendicular to its easy axis. Figure S3 shows that this occurs for $H_u \approx 500$ Oe, which corresponds to an energy of $mH_u \approx 2\,\mathrm{neV}$, where $m$ is the magnetic moment per unit cell [9]. We note that this simple estimate ignores the effect of the fourfold anisotropy ($\sim$1 neV [9]). Nevertheless, it gives an approximate upper bound for the uniaxial anisotropy energy scale near 295 K.

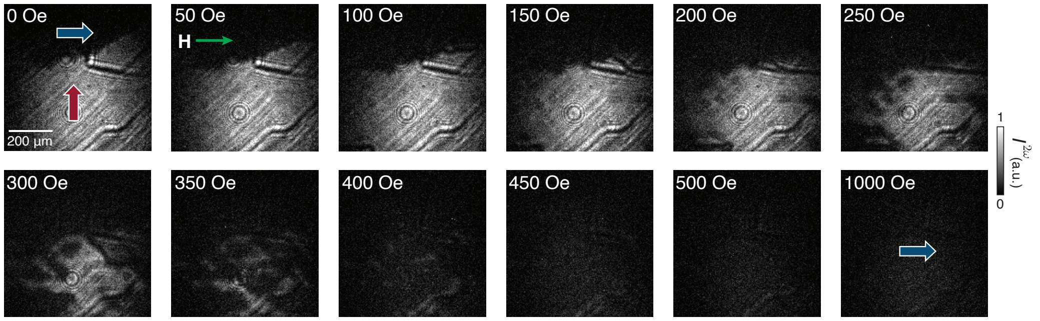


FIG. S3. SHG images at select magnetic fields applied along the magnetization direction of the dark domain. Images acquired with horizontal excitation polarization.

## 6. Comparison to conclusions drawn from prior magnetization experiments

It was originally proposed that the domain wall stability and dynamics in $Sr_2Cu_3O_4Cl_2$ may originate from entropy considerations [10], which can energetically favor the creation of domain walls. However, this explanation relies on there being interactions between many domain walls. Our SHG imaging experiments clearly show that the samples contain very few domain walls, so entropic terms cannot play a central role in the domain wall stability or magnetic field dependence. Instead, we have shown that the domain formation is controlled by a spatially dependent uniaxial anisotropy.

Subsequent theoretical work proposed that domain wall stability may be controlled by magnetoelastic effects that cause intrinsic internal stresses in antiferromagnets [11]. The stresses can then give rise to an in-plane uniaxial magnetic anisotropy, consistent with our observations. However, this intrinsic "de-stressing" effect should depend on the sample shape, and it is expected that samples with a square or rectangular shape possess a domain morphology that is regular and periodic in order to minimize the de-stressing energy [12]. The antiferromagnetic domains we observe do not show this regularity (Fig. S2). Furthermore, while de-stressing effects can give rise to a divergent domain wall susceptibility, it is not clear how they can produce domain-dependent spin reorientation. Therefore, intrinsic crystallographic distortions or inhomogeneous stresses from defects likely play a more important role in stabilizing the antiferromagnetic domains in $Sr_2Cu_3O_4Cl_2$. Based on the thermal cycling data in Section 4, these structural inhomogeneities should exist even above $T_{\mathrm{N,I}}$. Further work is needed to better understand their microscopic nature.

In ref. [10], a Landau theory was used to explain the low-field magnetization behavior of $Sr_2Cu_3O_4Cl_2$. They found that the divergent magnetic susceptibility arises when the parameter $a \to 0$. However, the magnetization data show very similar behavior above and below $T_{\mathrm{R}}$, which does not agree with the theory if it is assumed that $a$ crosses through zero (i.e., $a > 0$ for $T > T_{\mathrm{R}}$ and $a < 0$ for $T < T_{\mathrm{R}}$). Our temperature-dependent SHG imaging data (Fig. 3a) show that the domains A and B effectively swap their magnetic moments across $T_{\mathrm{R}}$. This symmetry in the domain structure above and below $T_{\mathrm{R}}$ implies that the potential energy landscape should be very similar above and below $T_{\mathrm{R}}$, so $a$ should reach a minimum at $T = T_{\mathrm{R}}$ instead of changing sign. Our work therefore further constrains the theory of ref. [10]. Moreover, our finding that the spin reorientation controls the divergent susceptibility suggests that $a$ must be related to the in-plane uniaxial anisotropy.

### 7. Full temperature dependence of magnetic domains

Figure S4 shows the magnetic domain structure temperature dependence. At intermediate temperatures, there is significant thermal hysteresis. In general, at lower temperatures, the crystal prefers a domain structure with smooth walls and a few large domains, which is consistent with exchange dominating relative to the anisotropy.

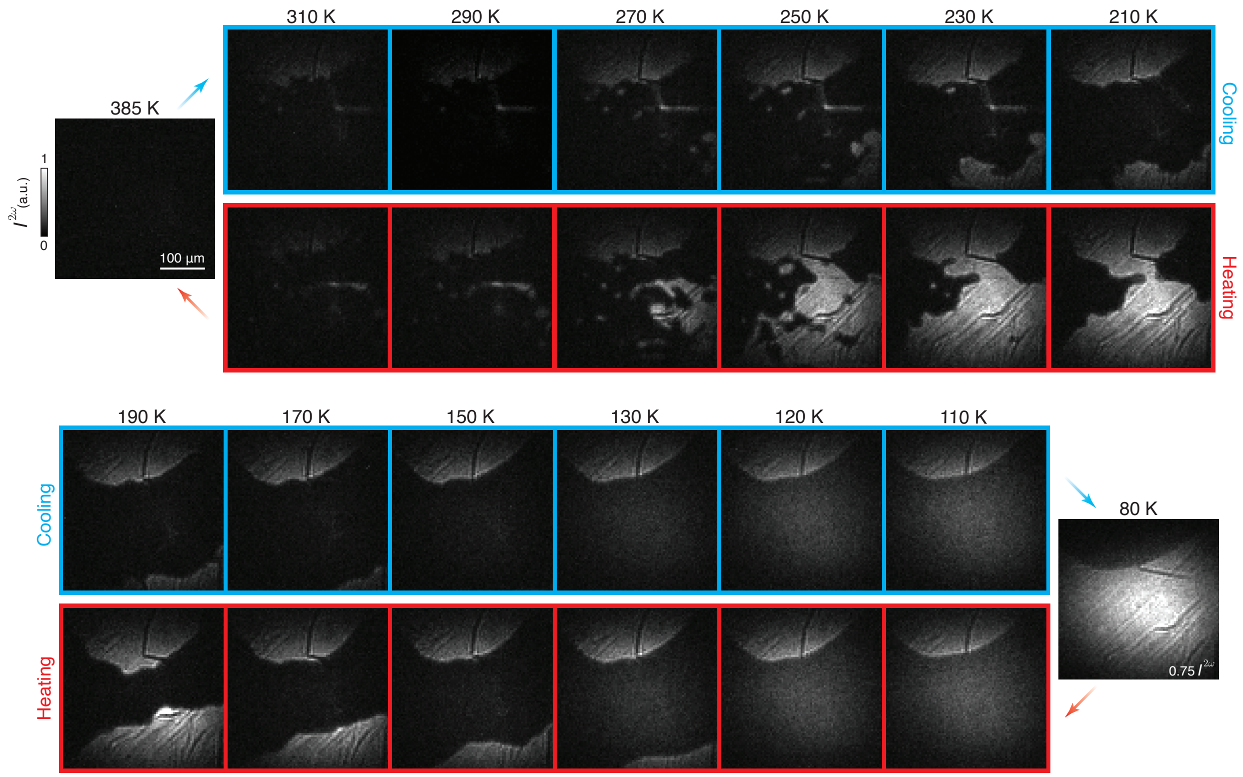


FIG. S4. Temperature-dependent SHG imaging starting from 385 K (top left), cooling (1st and 3rd rows, blue shading) to 80 K (bottom right), and then heating (4th and 2nd rows) back to 385 K. Significant thermal hysteresis is seen between approximately 130 K and 270 K. Images are acquired with vertical excitation polarization, so bright (dark) regions correspond to horizontal (vertical) magnetization direction. All images are plotted on the same color scale except for the 80 K image intensity, which was scaled down by 25 %.

### 8. Observation of domain reorientation transition in an additional sample

Figure S5 explores SHG imaging on an additional sample, which shows the same essential features as the main sample. In particular, there exist magnetic domains with a relative orientation of 90°. The 90° domain wall becomes smoother at low temperatures. And when heating or cooling through ∼100 K, the sample becomes a single magnetic domain followed by a 90° domain reorientation with the domain wall position unchanged.

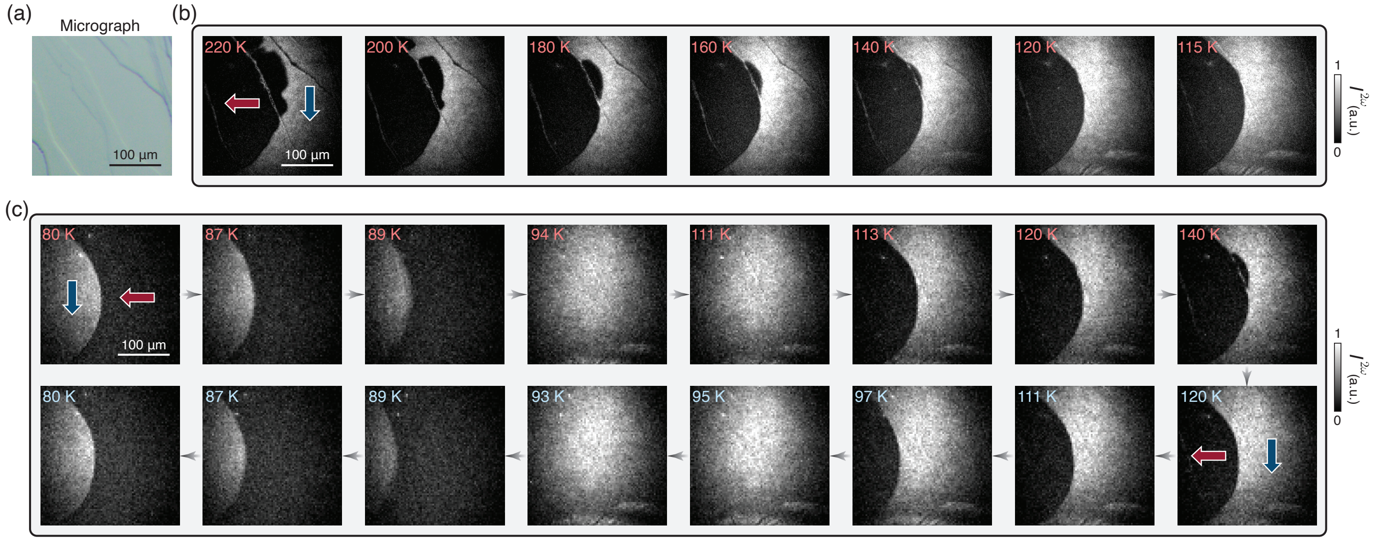


FIG. S5. **a**, Bright-field optical micrograph. **b**, SHG images at different temperatures showing the evolution of the 90° domain wall. Images acquired with horizontal excitation polarization. The bright and dark lines are due to the variation in scattering off terrace steps. **c**, Temperature dependence of the magnetic domains heating from 80 K to 140 K (top row) and cooling back to 80 K (bottom row). Red and blue arrows show the magnetization directions given by local RA-SHG measurements.

### 9. Field-direction dependence of single-domain magnetization near $T_R$

Figure S6 shows SHG images taken while thermally cycling through $T_R$ in the presence of a weak applied magnetic field. The magnetization direction of the single-domain state at $T_R$ is determined by the orientation of the applied field. This allows the preparation of a large-area (sample-sized, $\sim$1 $mm^2$ in this case) single-domain antiferromagnet.

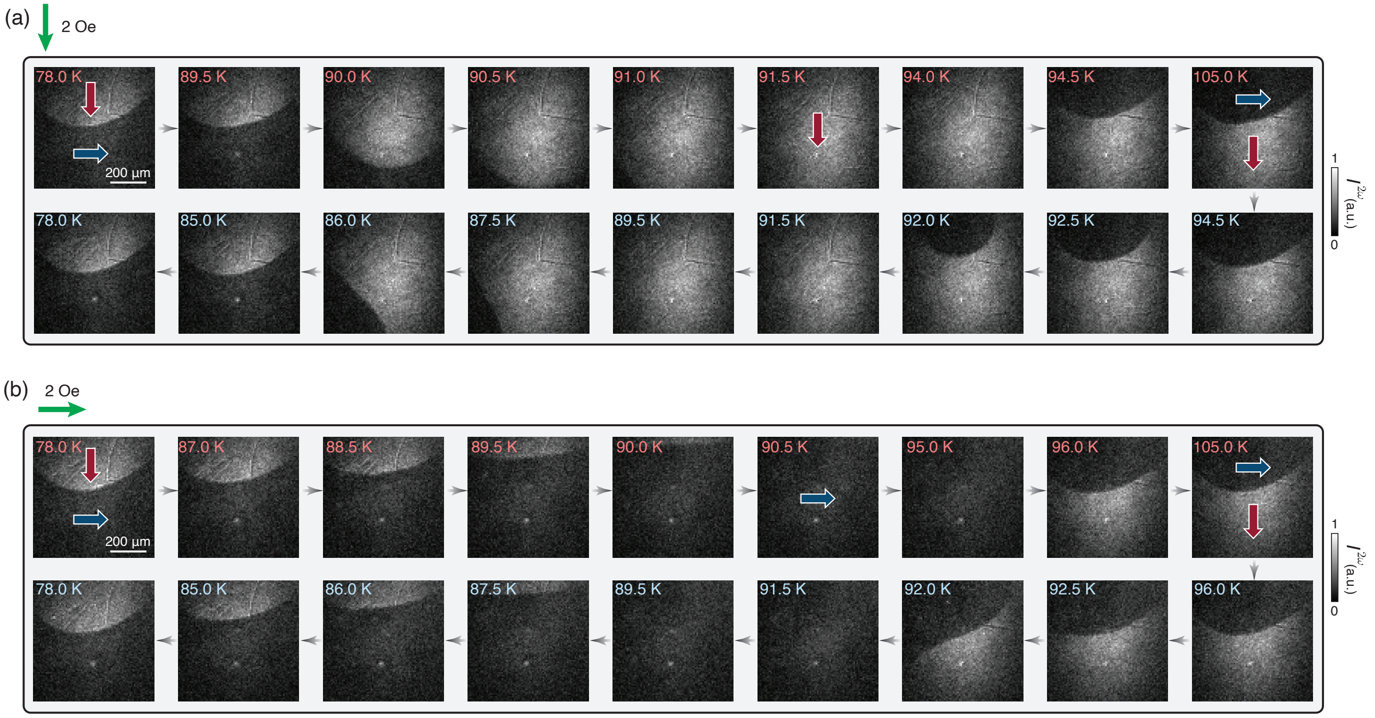


FIG. S6. Temperature dependence of magnetic domains at selected temperatures across the $T_R$ transition with an applied magnetic field of 2 Oe in the downward, **a**, or rightward, **b**, directions. The single-domain state close to $T_R$ possesses magnetization in the downward (rightward) directions for **a** (**b**), as confirmed by local RA-SHG measurements. Images acquired with horizontal excitation polarization.

[1] S. Noro, T. Kouchi, H. Harada, T. Yamadaya, M. Tadokoro, and H. Suzuki, Magnetic properties of $Ba_2Cu_3O_4Cl_2$ single crystals, Mater. Sci. Eng. B **25**, 167 (1994).

[2] J. W. Harter, L. Niu, A. J. Woss, and D. Hsieh, High-speed measurement of rotational anisotropy nonlinear optical harmonic generation using position-sensitive detection, Opt. Lett. **40**, 4671 (2015).

[3] A. de la Torre, K. L. Seyler, L. Zhao, S. D. Matteo, M. S. Scheurer, Y. Li, B. Yu, M. Greven, S. Sachdev, M. R. Norman, and D. Hsieh, Mirror symmetry breaking in a model insulating cuprate, Nat. Phys. **17**, 777 (2021).

[4] A. de la Torre, S. Di Matteo, D. Hsieh, and M. R. Norman, Implications of second harmonic generation for hidden order in $Sr_2CuO_2Cl_2$, Phys. Rev. B **104** (2021).

[5] R. R. Birss, *Symmetry and magnetism* (North-Holland Pub. Co., 1964).

[6] J. Reif, J. C. Zink, C. Schneider, and J. Kirschner, Effects of surface magnetism on optical second harmonic generation, Phys. Rev. Lett. **67**, 2878 (1991).

[7] A. Kirilyuk and T. Rasing, Magnetization-induced-second-harmonic generation from surfaces and interfaces, J. Opt. Soc. Am. B, JOSAB **22**, 148 (2005).

[8] K. L. Seyler, A. de la Torre, Z. Porter, E. Zoghlin, R. Polski, M. Nguyen, S. Nadj-Perge, S. D. Wilson, and D. Hsieh, Spin-orbit-enhanced magnetic surface second-harmonic generation in $Sr_2IrO_4$, Phys. Rev. B **102**, 201113 (2020).

[9] F. C. Chou, A. Aharony, R. J. Birgeneau, O. Entin-Wohlman, M. Greven, A. B. Harris, M. A. Kastner, Y. J. Kim, D. S. Kleinberg, Y. S. Lee, and Q. Zhu, Ferromagnetic moment and spin rotation transitions in tetragonal antiferromagnetic $Sr_2Cu_3O_4Cl_2$, Phys. Rev. Lett. **78**, 535 (1997).

[10] B. Parks, M. A. Kastner, Y. J. Kim, A. B. Harris, F. C. Chou, O. Entin-Wohlman, and A. Aharony, Magnetization measurements of antiferromagnetic domains in $Sr_2Cu_3O_4Cl_2$, Phys. Rev. B **63**, 134433 (2001).

[11] H. V. Gomonay, I. G. Korniienko, and V. M. Loktev, Theory of magnetization in multiferroics: Competition between ferromagnetic and antiferromagnetic domains, Phys. Rev. B **83**, 054424 (2011).

[12] H. V. Gomonay and V. M. Loktev, Shape-induced phenomena in finite-size antiferromagnets, Phys. Rev. B **75**, 174439 (2007).
